# Supplementary material for: MultiVENT: Multilingual Videos of Events with Aligned Natural Text
Source: arXiv:2307.03153 source file (2023-07-06)
Supplement: Supplementary file 1 [file appendix.tex]

\section{Current events}
\begin{table*}[t]
\tiny
 \centering
  \begin{tabular}{|c|ccccc|}
  \hline
    & Arabic & Chinese & English & Korean & Russian \\
  \hline
    Disasters & Fire in Ataba Market & Luding Earthquake & Flooding in Las Vegas & Flooding in South Korea & Soyuz Pipeline Leak \\
    & Flooding in Medina & Fire in Shanghai & Fires in Oregon & Daegu Office Fire & Fire in Cafe Polygon \\
    & Flooding in Jeddah & Three Gorges Dam Flood &  &  &  \\
    & Violence in Kabul &  &  &  &  \\
    & Cyprus Earthquake &  &  &  &  \\
    & Cyclone Shasheen &  &  &  &  \\
    & Iraq Dust Storm &  &  &  &  \\
    & Beirut Explosion &  &  &  &  \\
    & EgyptAir Flight 804 &  &  &  &  \\
    & Fire in Lusail &  &  &  &  \\
    & Cairo Factory Fire &  &  &  &  \\
    & Sohag Train Collision &  &  &  &  \\
    & Riyadh Drone Attack &  &  &  &  \\
    \hline
    Social &  &  &  &  &  \\
        &  &  &  &  &  \\
    &  &  &  &  &  \\
    &  &  &  &  &  \\
    &  &  &  &  &  \\
    &  &  &  &  &  \\
    &  &  &  &  &  \\
    &  &  &  &  &  \\
    &  &  &  &  &  \\
    &  &  &  &  &  \\
    &  &  &  &  &  \\
    &  &  &  &  &  \\
    &  &  &  &  &  \\
    \hline
    Political &  &  &  &  &  \\
        &  &  &  &  &  \\
    &  &  &  &  &  \\
    &  &  &  &  &  \\
    &  &  &  &  &  \\
    &  &  &  &  &  \\
    &  &  &  &  &  \\
    &  &  &  &  &  \\
    &  &  &  &  &  \\
    &  &  &  &  &  \\
    &  &  &  &  &  \\
    &  &  &  &  &  \\
    &  &  &  &  &  \\
    \hline
    Technology &  &  &  &  &  \\
        &  &  &  &  &  \\
    &  &  &  &  &  \\
    &  &  &  &  &  \\
    &  &  &  &  &  \\
    &  &  &  &  &  \\
    &  &  &  &  &  \\
    &  &  &  &  &  \\
    &  &  &  &  &  \\
    &  &  &  &  &  \\
    &  &  &  &  &  \\
    &  &  &  &  &  \\
    &  &  &  &  &  \\
    \hline
  \end{tabular}
  \caption{Ex}
  \label{tab:1}
\end{table*}

\begin{table*}[t]
 \centering
  \begin{tabular}{|cccc|}
  \hline
  Disasters & Social & Political & Technology \\
  \hline
      &  &  &  \\
    \hline
  \end{tabular}
  \caption{Ex}
  \label{tab:1}
\end{table*}
